# Supplementary material for: Invariance of Immersed Floer cohomology under Maslov flows
Source: arXiv:1804.06799 source file (2026-04-03)

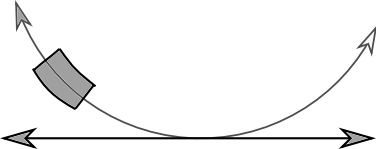

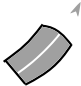

Supplement: Supplementary file 1 [file supp.pdf]
